# Supplementary material for: Neural Kernel Surface Reconstruction
Source: arXiv:2305.19590 source file (2023-06-09)

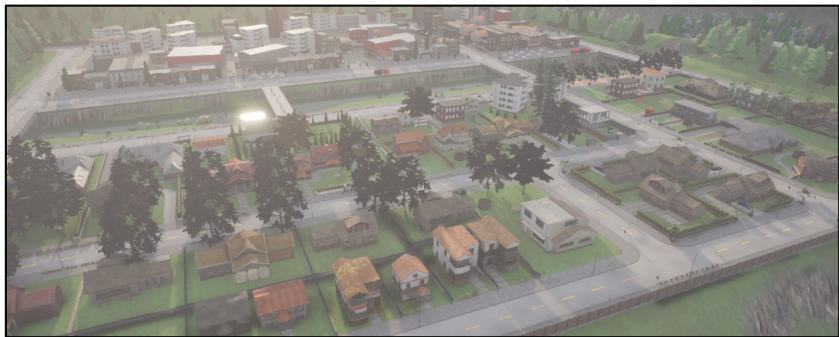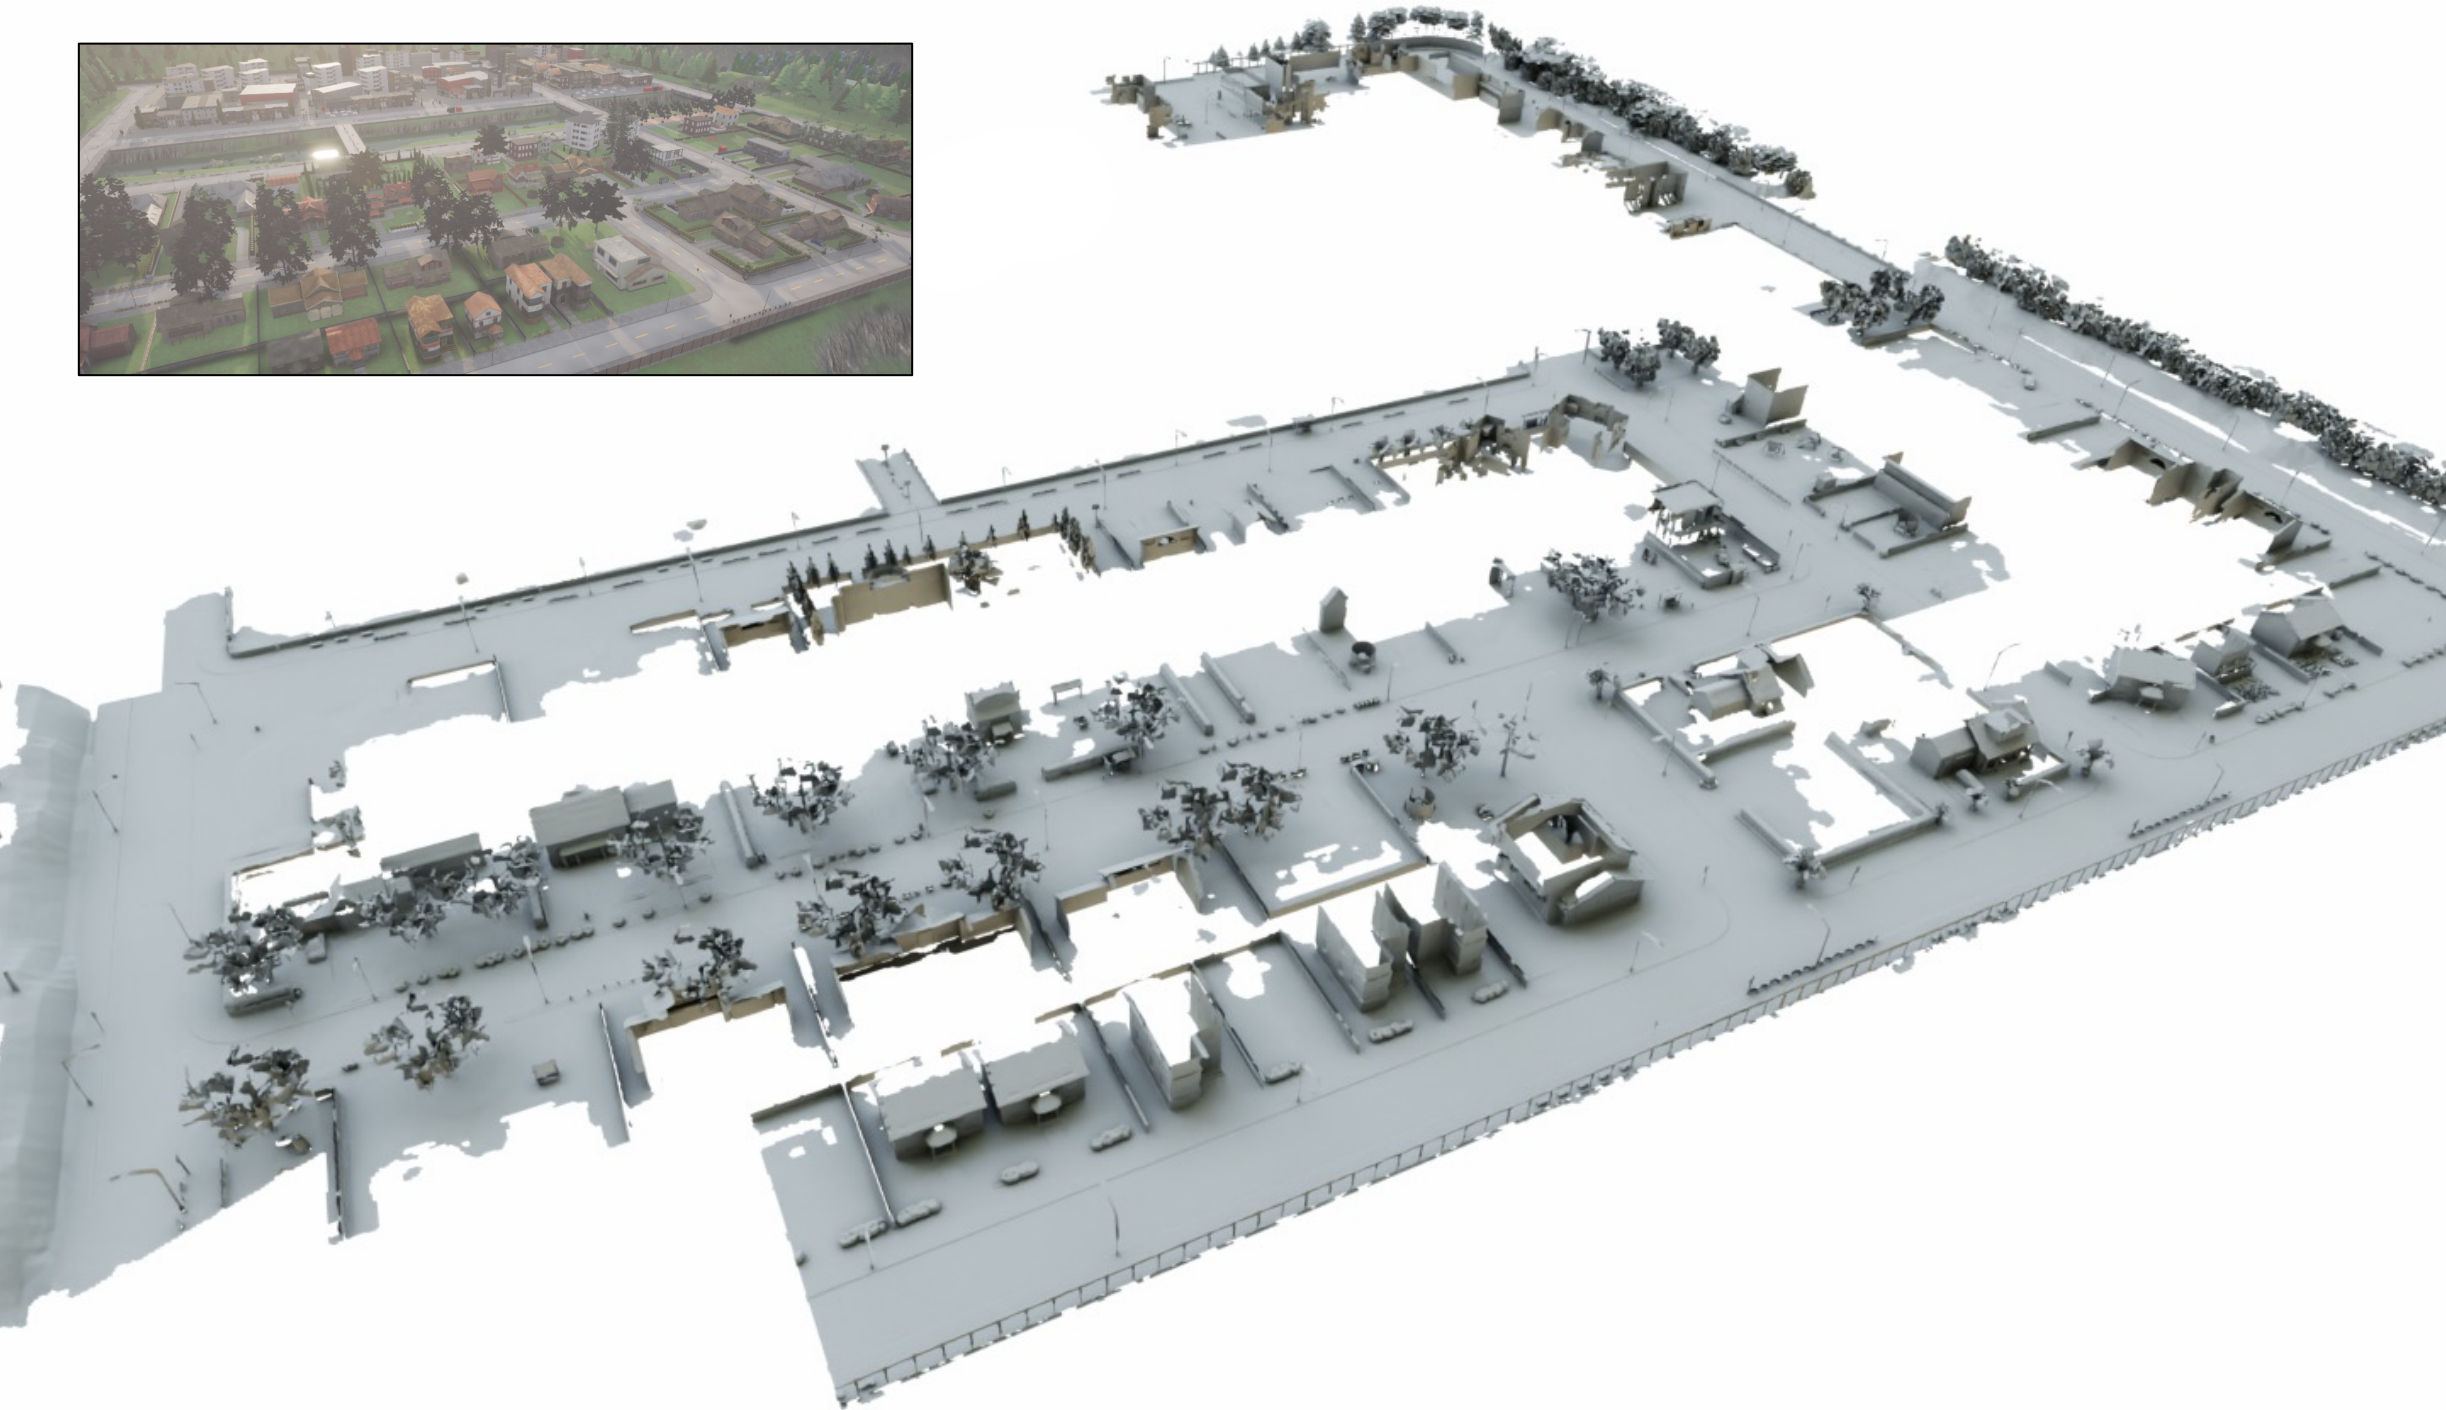

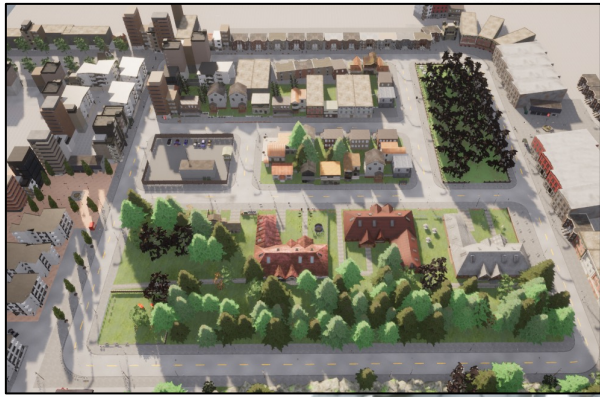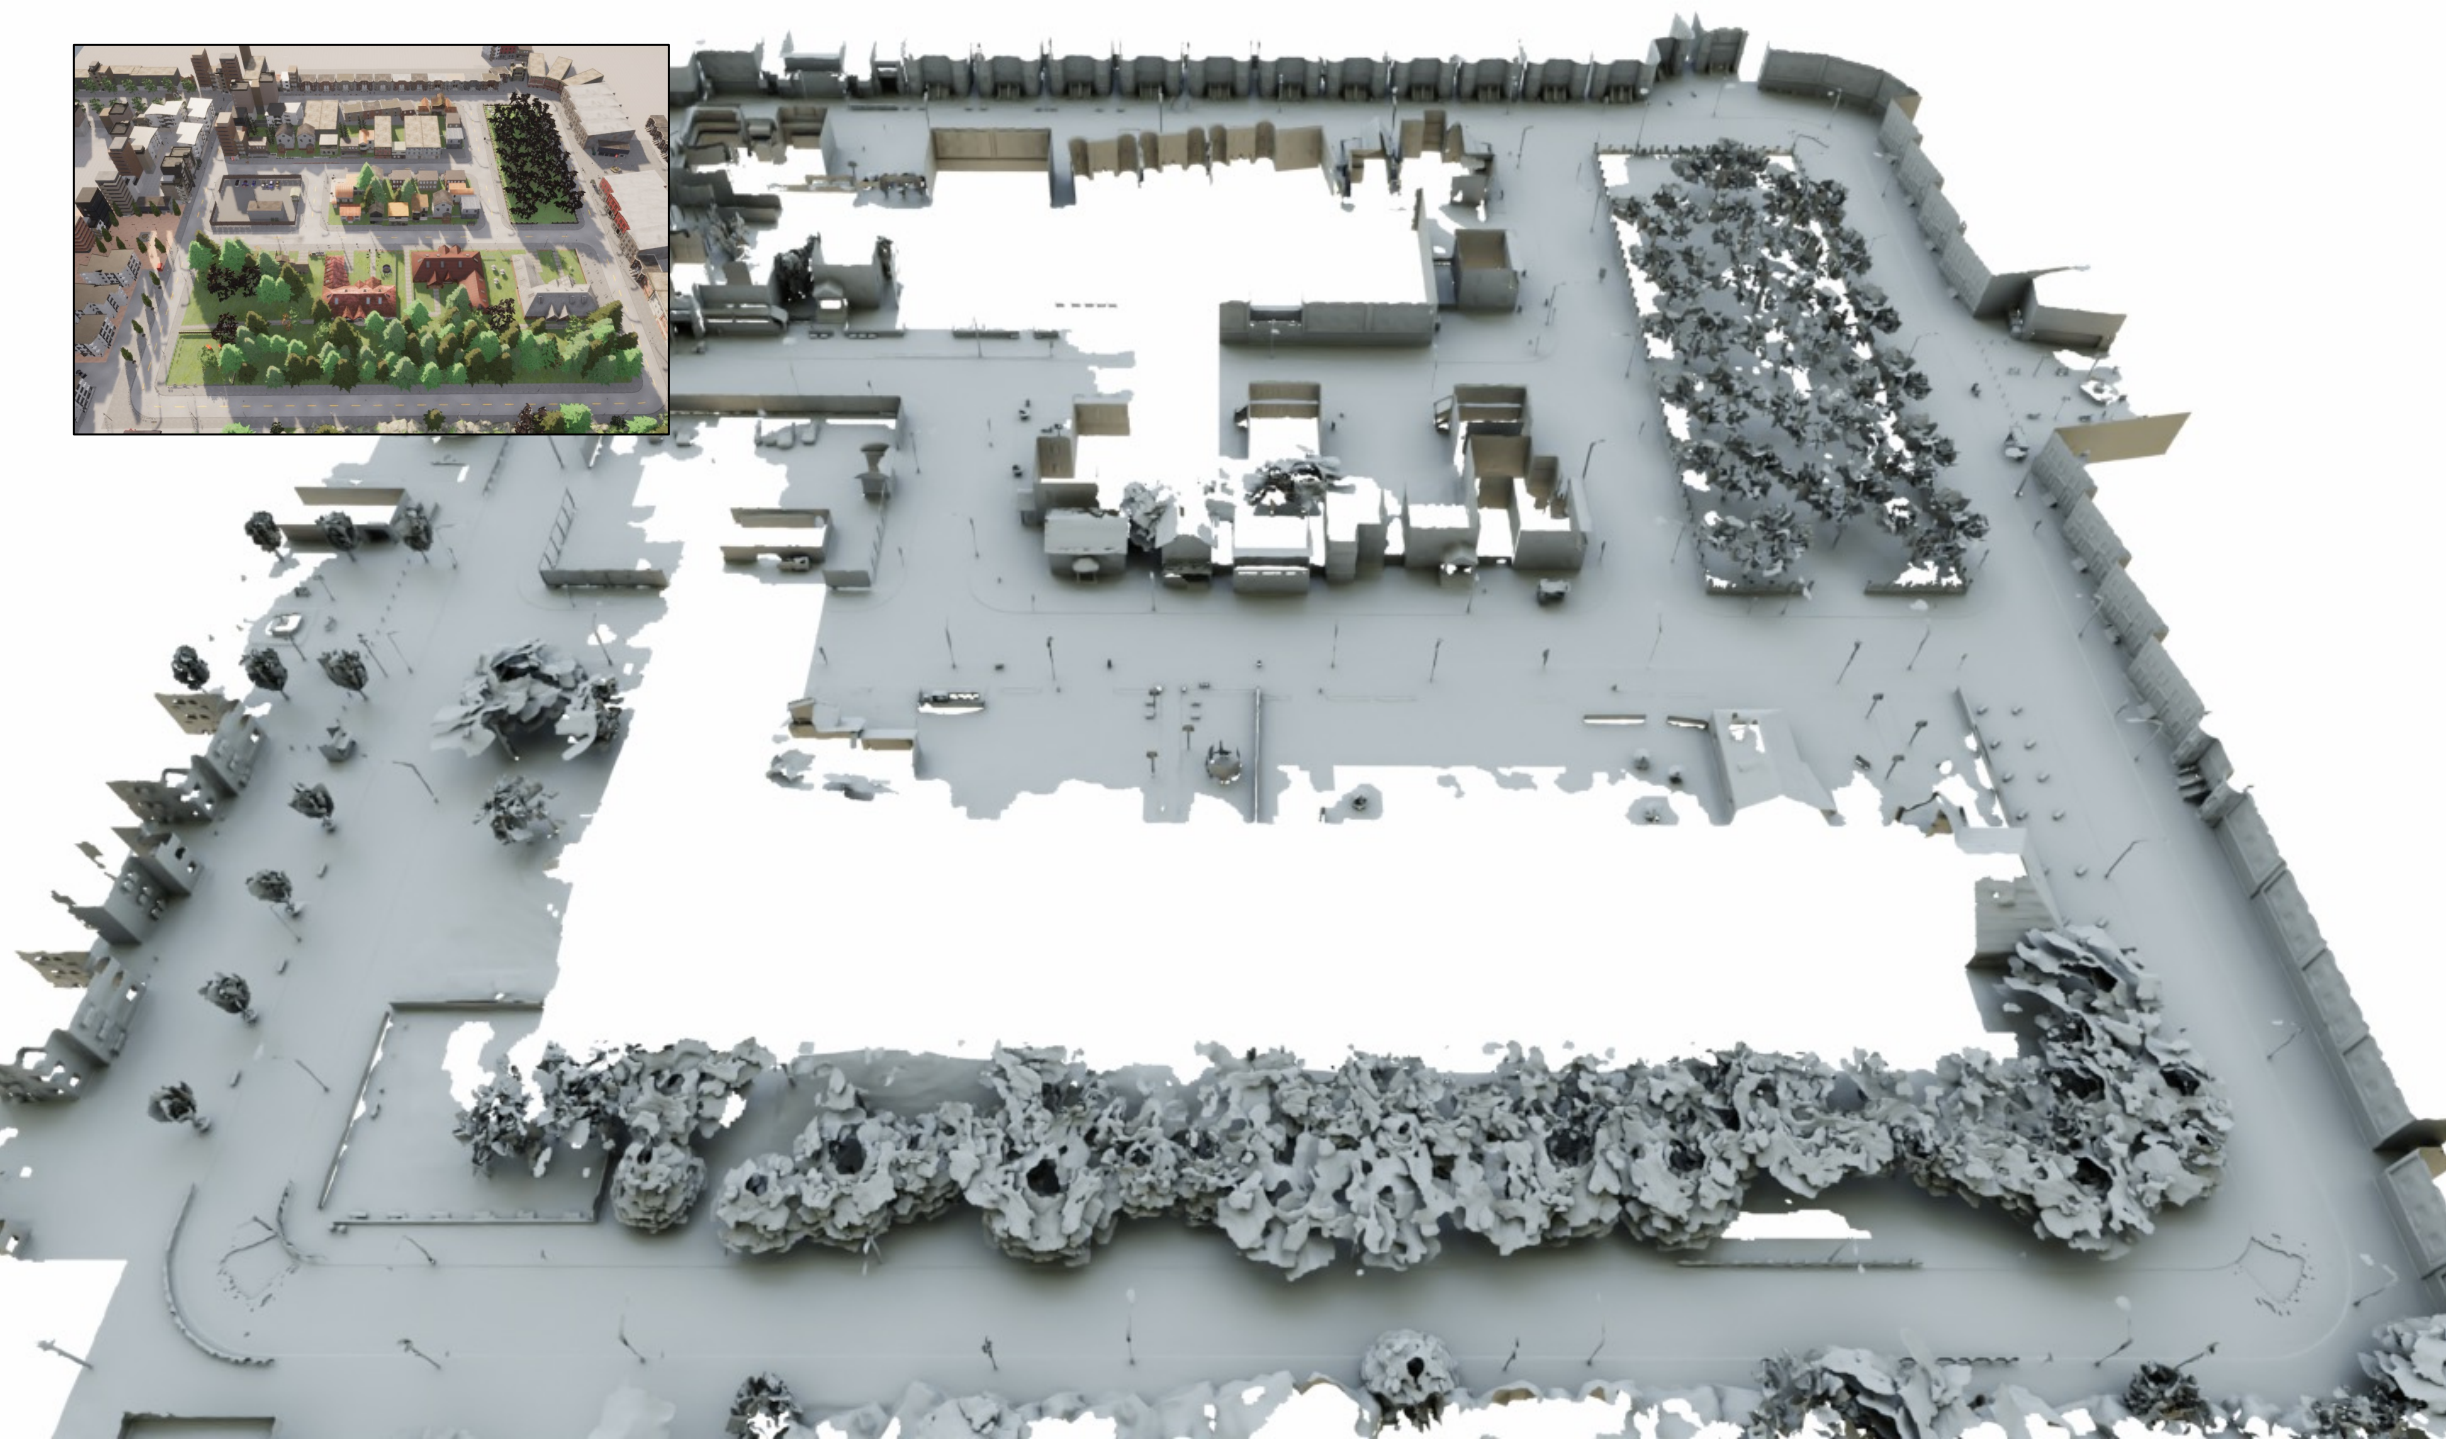

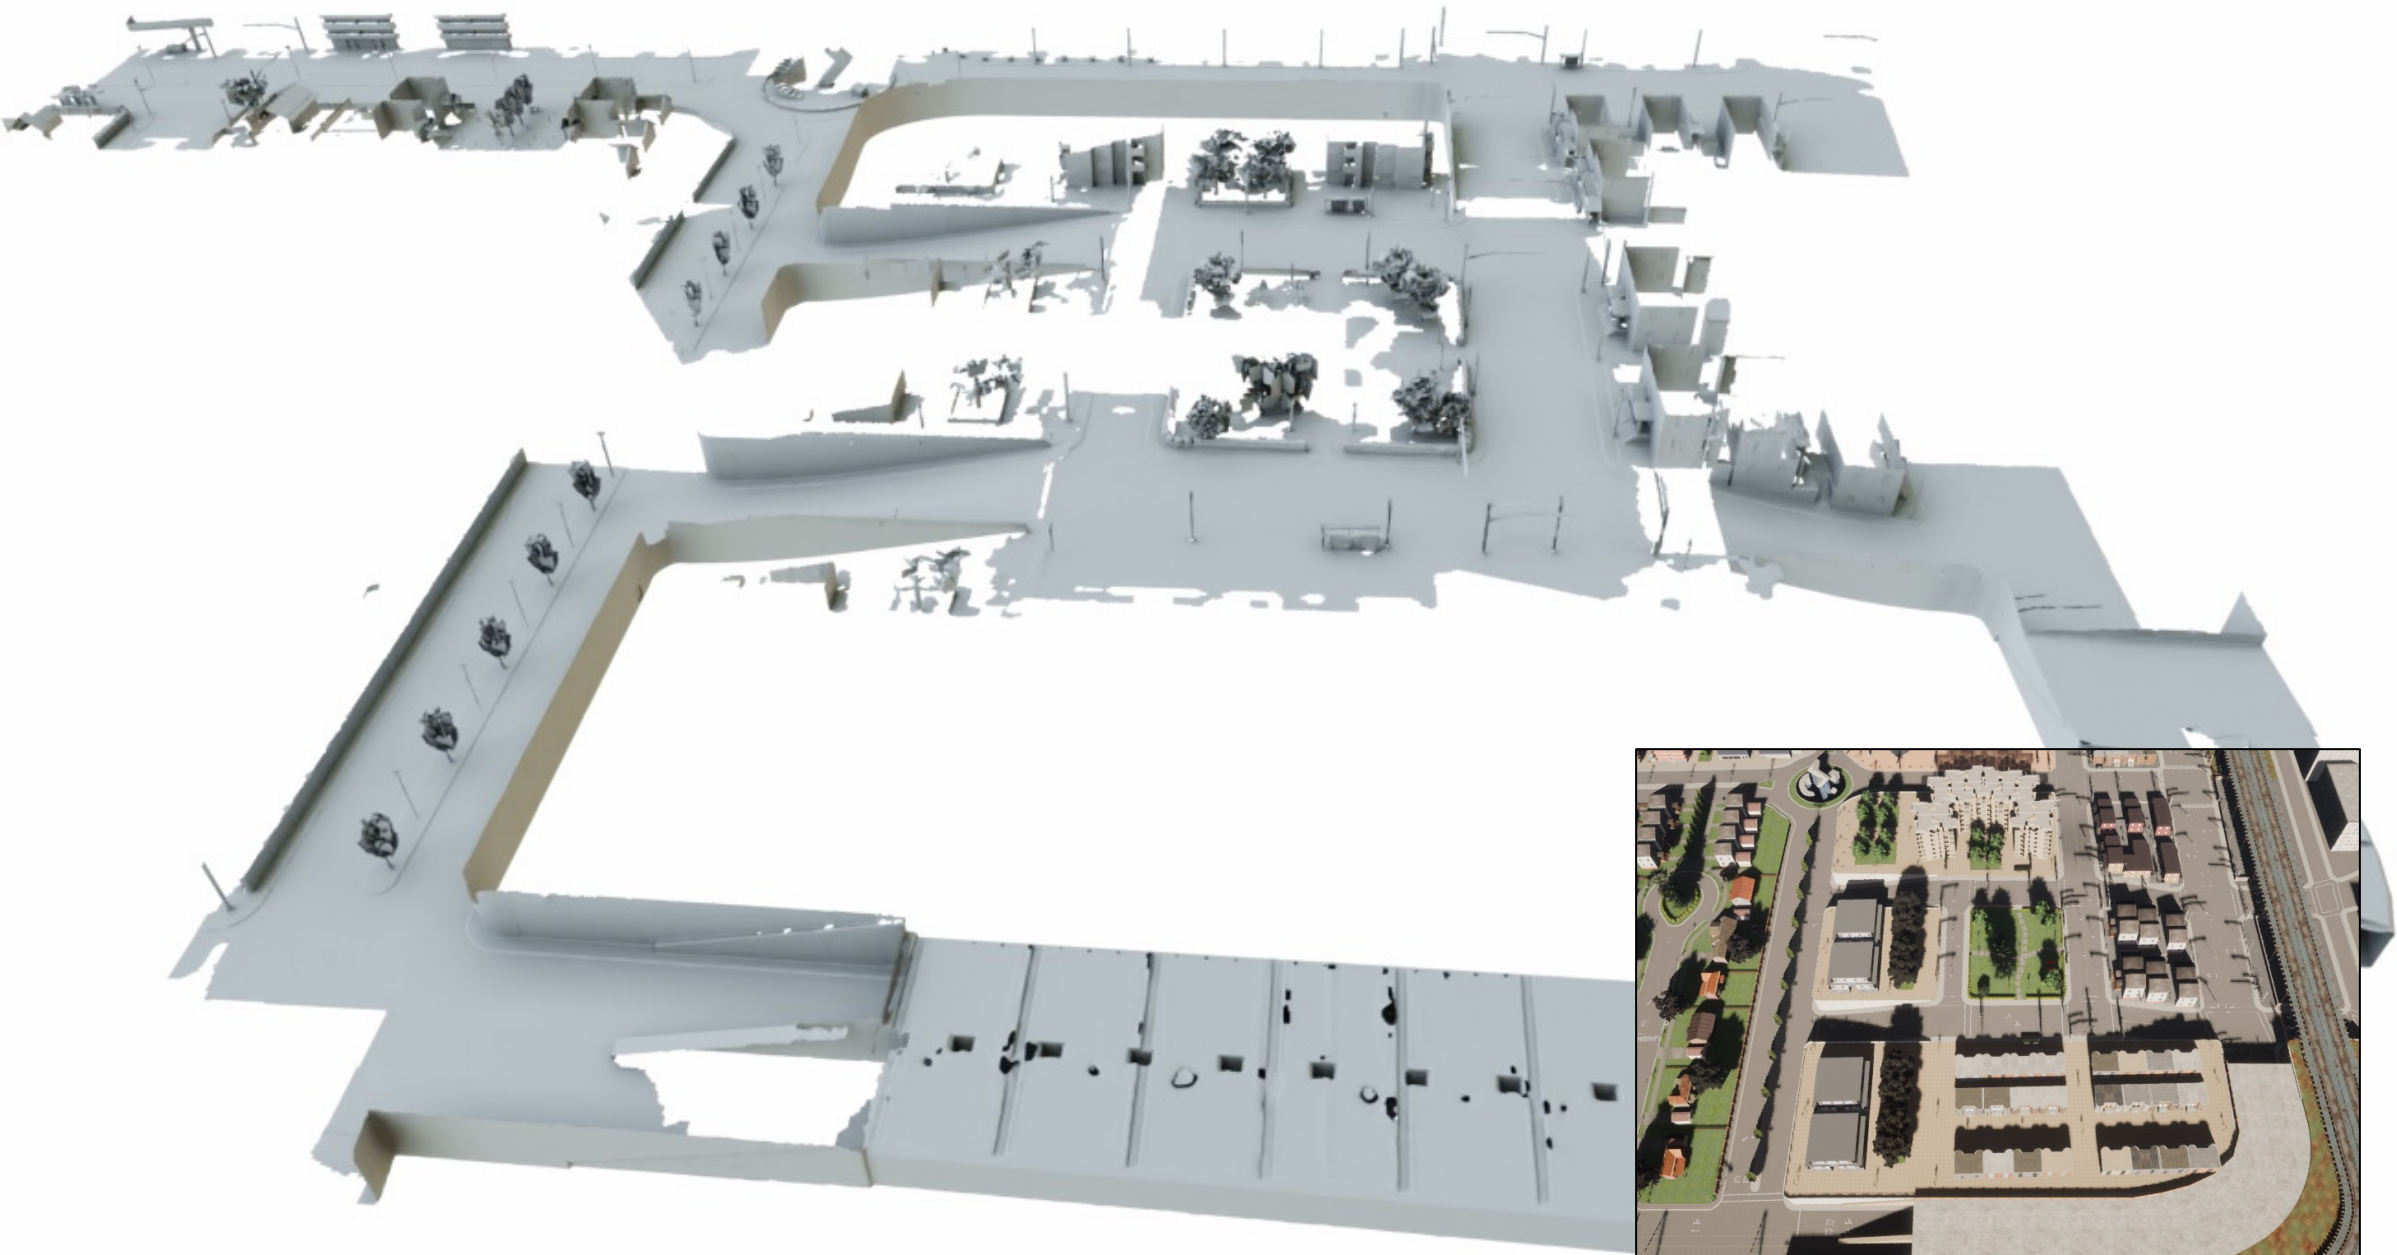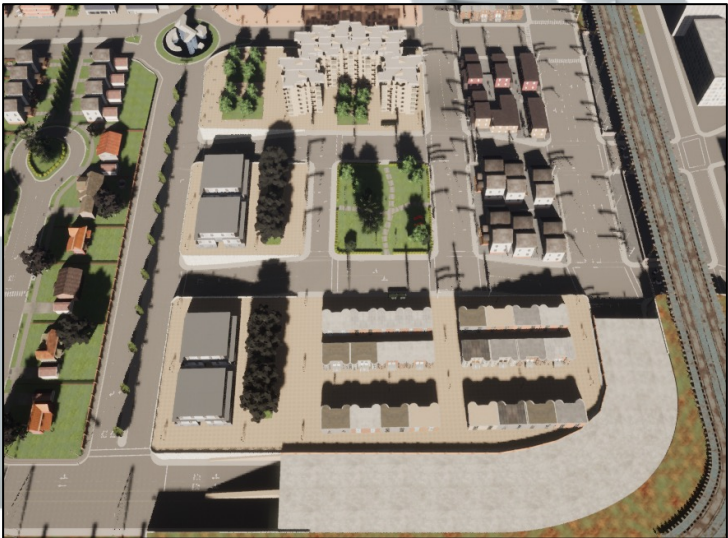

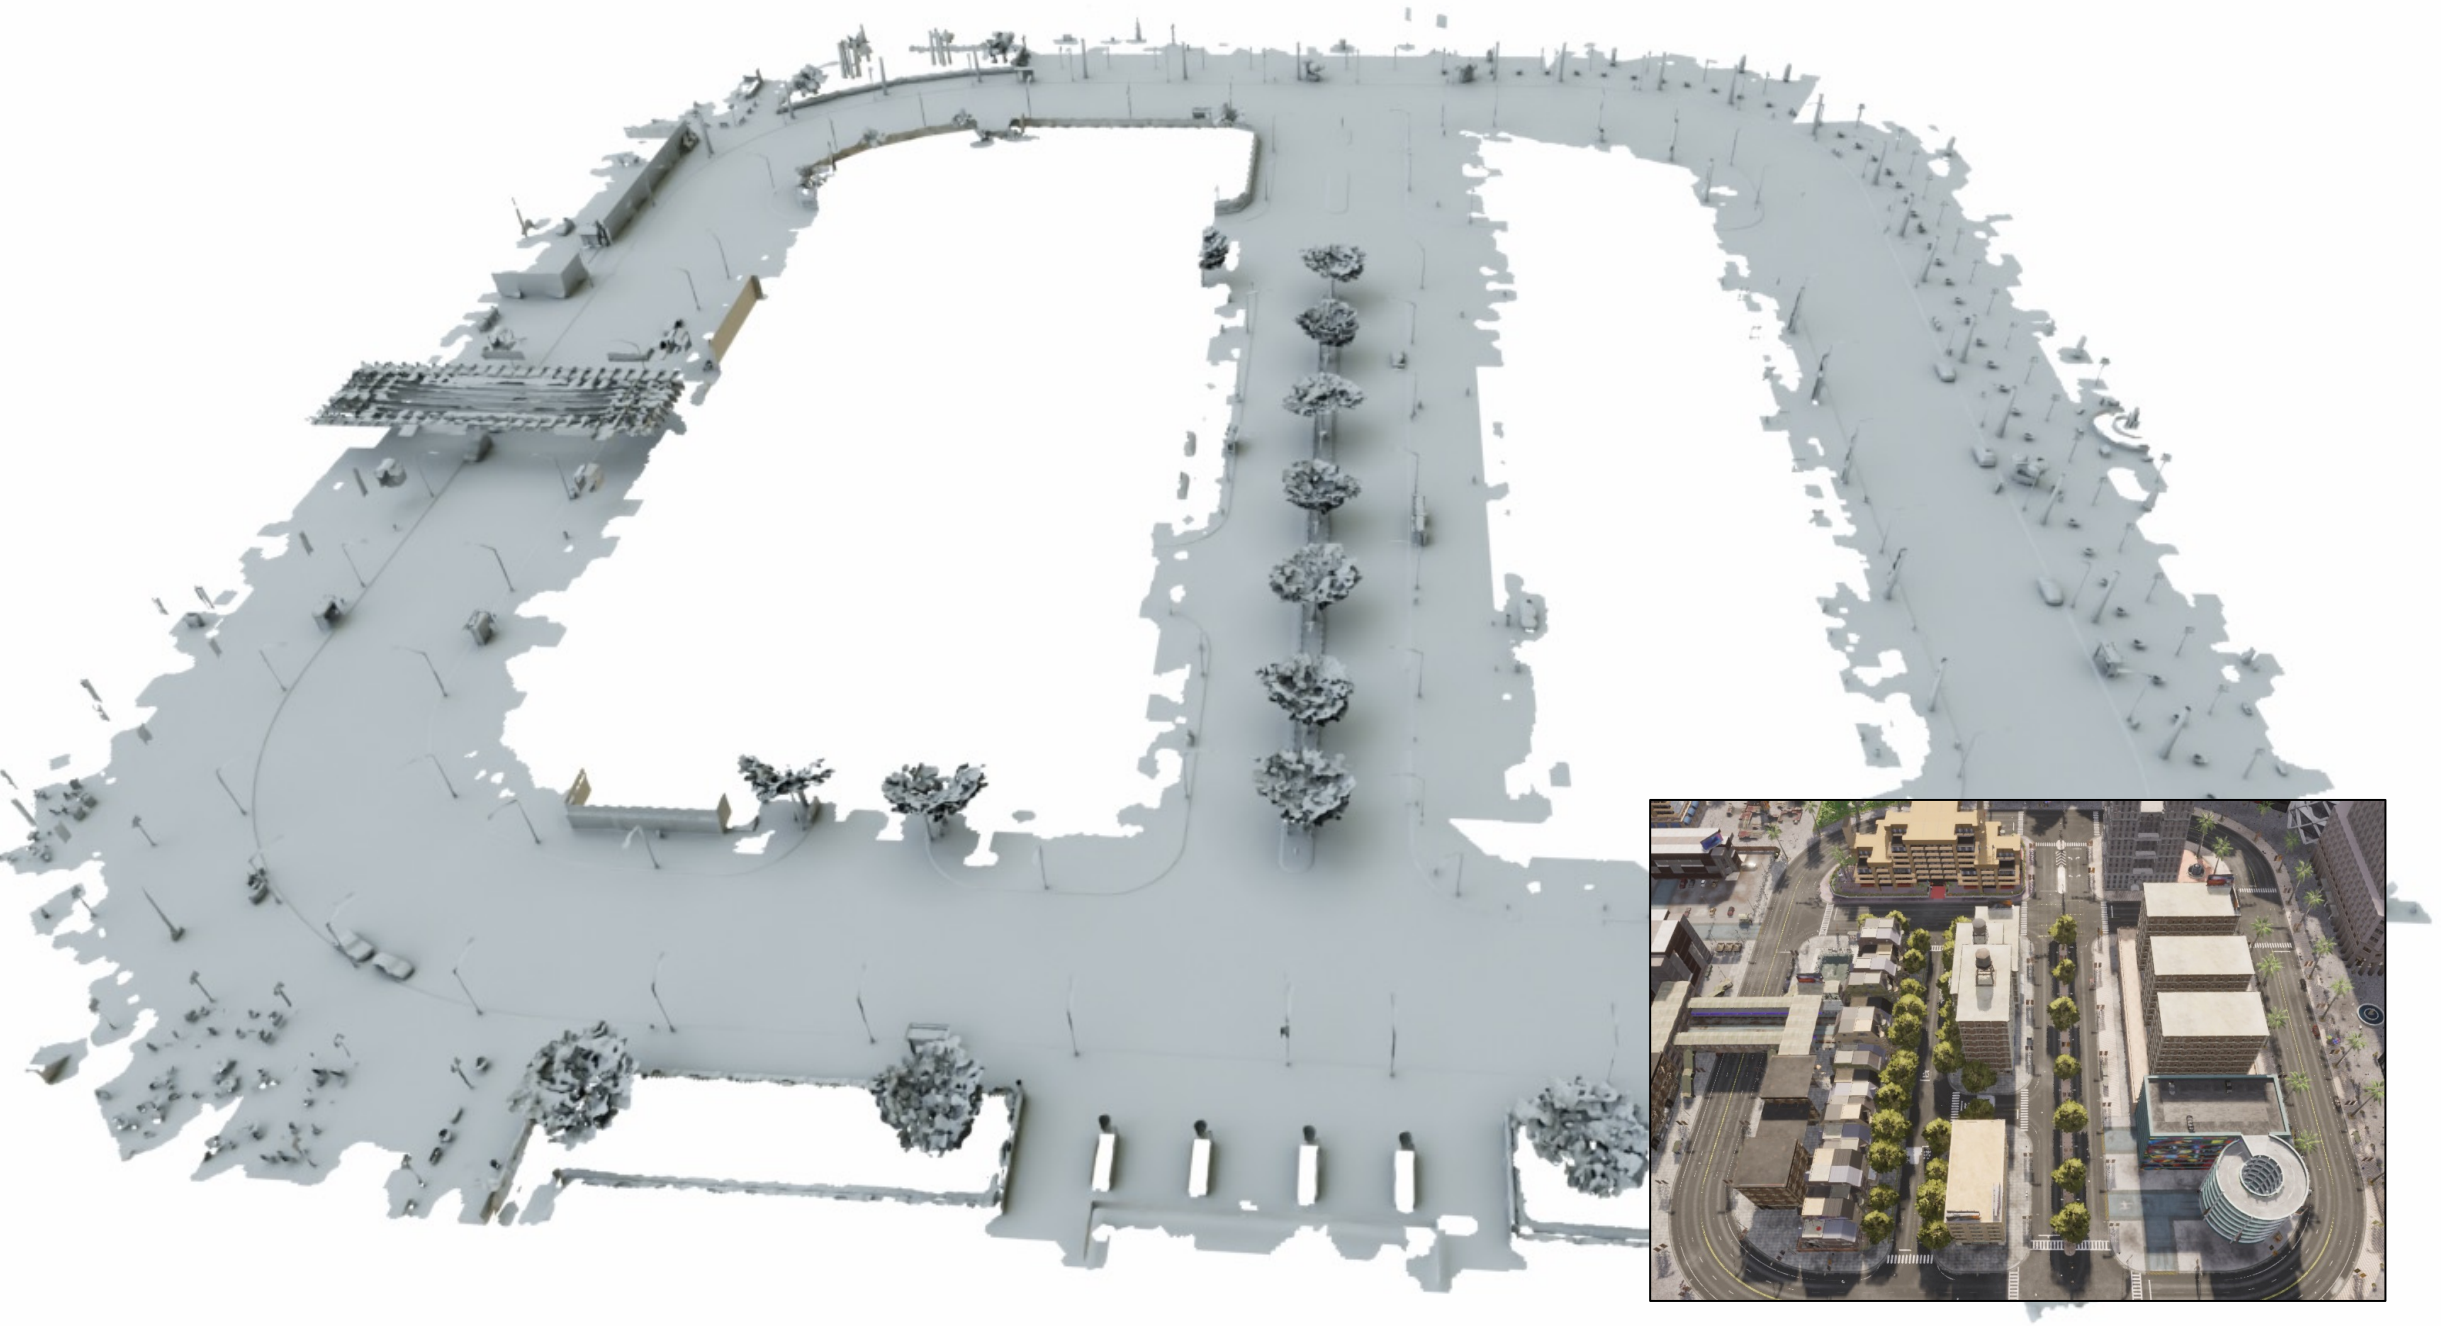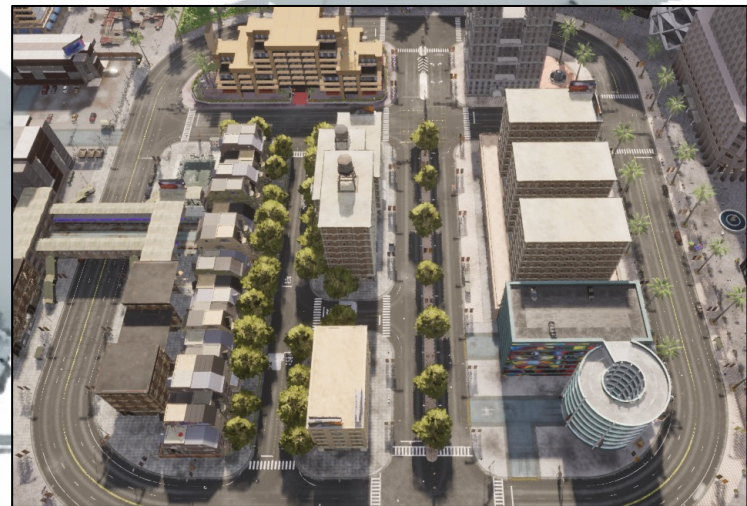

Supplement: Supplementary file 1 [file supp-carla.pdf]
